# Supplementary material for: A Benchmarking Study of Matching Algorithms for Knowledge Graph Entity Alignment
Source: arXiv:2308.03961 source file (2023-08-08)
Supplement: Supplementary file 1 [file appendix.tex]

\appendix

\section{Comparative results for threshold=0}
\begin{table*}[!ht]
    \caption{F1-score at threshold=0.0. Note that F1-score of Greedy == Hit@1. \cite{mao_alignment_2021} uses \cite{mena_sinkhorn_approx_2018} while \cite{zeng_matching_benchmarking_2023} uses \cite{cuturi_sinkhorn_distance_2013}.}
    \label{tab:performance_prf1_00}
    \setlength{\tabcolsep}{3.5pt}
    \begin{tabular}{|ll|ccc|ccc|ccc|ccc|ccc|ccc|ccc|}
        \toprule
         &  & \multicolumn{9}{c|}{DBP15K} & \multicolumn{12}{c|}{SRPRS} \\
         \cline{3-23}
         &  & \multicolumn{3}{c|}{FR\_EN} & \multicolumn{3}{c|}{JA\_EN} & \multicolumn{3}{c|}{ZH\_EN} & \multicolumn{3}{c|}{EN\_FR} & \multicolumn{3}{c|}{EN\_DE} & \multicolumn{3}{c|}{DBP\_WD} & \multicolumn{3}{c|}{DBP\_YG} \\
         % \cline{3-23}
         &  & P & R & F1 & P & R & F1 & P & R & F1 & P & R & F1 & P & R & F1 & P & R & F1 & P & R & F1 \\
        \midrule
        \multirow[c]{7}{*}{\rotatebox[origin=c]{90}{PARIS}} & Native & 97.9 & 82.0 & 89.3 & 96.8 & 77.9 & 86.3 & 97.0 & 80.6 & 88.0 & 97.5 & 70.3 & 81.7 & 98.2 & 86.9 & 92.2 & 97.5 & 72.4 & 83.1 & 87.4 & 29.1 & 43.7 \\
         \cline{3-23}
         & DInf & 79.2 & 82.1 & 80.7 & 75.0 & 78.4 & 76.7 & 76.9 & 80.7 & 78.7 & 70.6 & 70.6 & 70.6 & 87.3 & 87.3 & 87.3 & 72.7 & 72.7 & 72.7 & 30.4 & 30.4 & 30.4 \\
         & Hun. & 80.1 & 83.0 & 81.6 & 77.6 & 80.9 & 79.2 & 78.7 & 82.6 & 80.6 & 74.9 & 74.9 & 74.9 & 89.8 & 89.8 & 89.8 & 77.3 & 77.3 & 77.3 & 38.1 & 38.1 & 38.1 \\
         & Sink-o & 71.4 & 74.0 & 72.7 & 70.4 & 73.5 & 71.9 & 70.5 & 74.0 & 72.2 & 70.5 & 70.5 & 70.5 & 85.9 & 85.9 & 85.9 & 73.5 & 73.5 & 73.5 & 33.2 & 33.2 & 33.2 \\
         & Sink-d & 77.0 & 79.8 & 78.3 & 74.3 & 77.6 & 75.9 & 76.0 & 79.7 & 77.8 & 74.1 & 74.1 & 74.1 & 88.1 & 88.1 & 88.1 & 76.1 & 76.1 & 76.1 & 37.2 & 37.2 & 37.2 \\
         & SMat & 87.4 & 90.6 & 89.0 & 81.7 & 85.2 & 83.4 & 83.0 & 87.2 & 85.1 & 76.2 & 76.2 & 76.2 & 91.0 & 91.0 & 91.0 & 78.0 & 78.0 & 78.0 & 37.8 & 37.8 & 37.8 \\
         & BMat & 94.4 & 90.6 & 92.5 & 92.1 & 85.2 & 88.5 & 93.1 & 87.1 & 90.0 & 80.9 & 76.2 & 78.5 & 94.2 & 91.0 & 92.6 & 85.6 & 78.1 & 81.7 & 45.4 & 37.9 & 41.3 \\
         \hline
        \multirow[c]{6}{*}{\rotatebox[origin=c]{90}{GCN-Align}} & DInf & 28.6 & 28.6 & 28.6 & 29.6 & 29.6 & 29.6 & 29.2 & 29.2 & 29.2 & 17.0 & 17.0 & 17.0 & 32.2 & 32.2 & 32.2 & 20.2 & 20.2 & 20.2 & 25.3 & 25.3 & 25.3 \\
         & Hun. & 48.5 & 48.5 & 48.5 & 48.0 & 48.0 & 48.0 & 45.0 & 45.0 & 45.0 & 24.7 & 24.7 & 24.7 & 38.6 & 38.6 & 38.6 & 28.5 & 28.5 & 28.5 & 33.0 & 33.0 & 33.0 \\
         & Sink-o & 19.6 & 19.6 & 19.6 & 22.0 & 22.0 & 22.0 & 20.3 & 20.3 & 20.3 & 14.4 & 14.4 & 14.4 & 20.9 & 20.9 & 20.9 & 17.0 & 17.0 & 17.0 & 18.7 & 18.7 & 18.7 \\
         & Sink-d & 48.4 & 48.4 & 48.4 & 47.8 & 47.8 & 47.8 & 44.7 & 44.7 & 44.7 & 24.8 & 24.8 & 24.8 & 38.8 & 38.8 & 38.8 & 28.9 & 28.9 & 28.9 & 33.1 & 33.1 & 33.1 \\
         & SMat & 38.8 & 38.8 & 38.8 & 41.9 & 41.9 & 41.9 & 38.2 & 38.2 & 38.2 & 23.1 & 23.1 & 23.1 & 37.1 & 37.1 & 37.1 & 26.0 & 26.0 & 26.0 & 31.2 & 31.2 & 31.2 \\
         & BMat & 38.8 & 38.8 & 38.8 & 41.9 & 41.9 & 41.9 & 38.2 & 38.2 & 38.2 & 23.1 & 23.1 & 23.1 & 37.1 & 37.1 & 37.1 & 26.0 & 26.0 & 26.0 & 31.2 & 31.2 & 31.2 \\
         \hline
        \multirow[c]{6}{*}{\rotatebox[origin=c]{90}{RREA}} & DInf & 62.8 & 62.8 & 62.8 & 60.3 & 60.3 & 60.3 & 60.5 & 60.5 & 60.5 & 36.7 & 36.7 & 36.7 & 52.1 & 52.1 & 52.1 & 41.6 & 41.6 & 41.6 & 44.8 & 44.8 & 44.8 \\
         & Hun. & 77.7 & 77.7 & 77.7 & 74.5 & 74.5 & 74.5 & 74.9 & 74.9 & 74.9 & 41.8 & 41.8 & 41.8 & 56.3 & 56.3 & 56.3 & 47.6 & 47.6 & 47.6 & 49.6 & 49.6 & 49.6 \\
         & Sink-o & 55.6 & 55.6 & 55.6 & 54.9 & 54.9 & 54.9 & 54.5 & 54.5 & 54.5 & 34.0 & 34.0 & 34.0 & 49.7 & 49.7 & 49.7 & 38.5 & 38.5 & 38.5 & 42.2 & 42.2 & 42.2 \\
         & Sink-d & 77.8 & 77.8 & 77.8 & 74.1 & 74.1 & 74.1 & 75.0 & 75.0 & 75.0 & 42.2 & 42.2 & 42.2 & 56.7 & 56.7 & 56.7 & 48.0 & 48.0 & 48.0 & 49.7 & 49.7 & 49.7 \\
         & SMat & 71.8 & 71.8 & 71.8 & 67.7 & 67.7 & 67.7 & 68.6 & 68.6 & 68.6 & 39.8 & 39.8 & 39.8 & 55.1 & 55.1 & 55.1 & 45.3 & 45.3 & 45.3 & 47.2 & 47.2 & 47.2 \\
         & BMat & 71.8 & 71.8 & 71.8 & 67.7 & 67.7 & 67.7 & 68.6 & 68.6 & 68.6 & 39.8 & 39.8 & 39.8 & 55.1 & 55.1 & 55.1 & 45.3 & 45.3 & 45.3 & 47.2 & 47.2 & 47.2 \\
        \bottomrule
    \end{tabular}
\end{table*}

\begin{table*}[!ht]
    \caption{F1-score for DWY100K at threshold=0.0}
    \label{tab:performance_prf1_00_100k}
    \begin{tabular}{|ll|ccc|ccc|}
        \toprule
         &  & \multicolumn{6}{c|}{DWY100K} \\
         \cline{3-8}
         &  & \multicolumn{3}{c|}{DBP\_WD} & \multicolumn{3}{c|}{DBP\_YG} \\
         &  & P & R & F1 & P & R & F1 \\
        \midrule
        \multirow[c]{7}{*}{\rotatebox[origin=c]{90}{PARIS}}
         & Native & 92.4 & 73.7 & 82.0 & 94.7 & 65.9 & 77.7 \\
         \cline{3-8}
         & DInf & 75.5 & 75.5 & 75.5 & 67.9 & 67.9 & 67.9 \\
         & Hun. & 79.5 & 79.5 & 79.5 & 80.1 & 80.1 & 80.1 \\
         & Sink-o & 74.7 & 74.7 & 74.7 & 70.9 & 70.9 & 70.9 \\
         & Sink-d & 78.8 & 78.8 & 78.8 & 79.0 & 79.0 & 79.0 \\
         & SMat & 81.3 & 79.6 & 80.4 & 79.1 & 77.4 & 78.2 \\
         & BMat & 82.9 & 79.5 & 81.1 & 79.8 & 77.4 & 78.6 \\
         \hline
        \multirow[c]{6}{*}{\rotatebox[origin=c]{90}{GCN-Align}}
         & DInf & 55.4 & 55.4 & 55.4 & 55.4 & 55.4 & 55.4 \\
         & Hun. & 73.6 & 73.6 & 73.6 & 73.6 & 73.6 & 73.6 \\
         & Sink-o & 33.5 & 33.5 & 33.5 & 33.5 & 33.5 & 33.5 \\
         & Sink-d & 74.0 & 74.0 & 74.0 & 74.0 & 74.0 & 74.0 \\
         & SMat & 66.6 & 66.6 & 66.6 & 66.6 & 66.6 & 66.6 \\
         & BMat & 66.6 & 66.6 & 66.6 & 66.6 & 66.6 & 66.6 \\
        \bottomrule
    \end{tabular}
\end{table*}
\begin{table*}[!ht]
    \caption{F1-score using name at threshold=0.0.}
    \label{tab:performance_name_00}
    \begin{tabular}{|ll|ccc|ccc|ccc|ccc|ccc|ccc|ccc|}
        \toprule
         &  & \multicolumn{9}{c|}{DBP15K} & \multicolumn{6}{c|}{SRPRS} \\
         \cline{3-17}
         &  & \multicolumn{3}{c|}{FR\_EN} & \multicolumn{3}{c|}{JA\_EN} & \multicolumn{3}{c|}{ZH\_EN} & \multicolumn{3}{c|}{EN\_FR} & \multicolumn{3}{c|}{EN\_DE} \\
         &  & P & R & F1 & P & R & F1 & P & R & F1 & P & R & F1 & P & R & F1 \\
        \midrule
        \multirow[c]{6}{*}{\rotatebox[origin=c]{90}{Sorensen-Dice}} & DInf & 65.4 & 85.7 & 74.2 & 57.4 & 75.8 & 65.3 & 48.7 & 62.9 & 54.9 & 90.3 & 90.3 & 90.3 & 89.7 & 89.7 & 89.7 \\
         & Hun. & 69.3 & 90.8 & 78.6 & 61.9 & 81.6 & 70.4 & 53.5 & 69.1 & 60.3 & 94.2 & 94.2 & 94.2 & 94.0 & 94.0 & 94.0 \\
         & Sink-o & 66.7 & 87.4 & 75.6 & 60.3 & 79.6 & 68.6 & 51.5 & 66.5 & 58.0 & 91.8 & 91.8 & 91.8 & 91.4 & 91.4 & 91.4 \\
         & Sink-d & 69.2 & 90.7 & 78.5 & 62.4 & 82.4 & 71.0 & 54.0 & 69.8 & 60.9 & 93.6 & 93.6 & 93.6 & 93.2 & 93.2 & 93.2 \\
         & SMat & 68.7 & 90.1 & 78.0 & 60.8 & 80.2 & 69.2 & 52.4 & 67.7 & 59.0 & 93.4 & 93.4 & 93.4 & 92.9 & 92.9 & 92.9 \\
         & BMat & 72.1 & 90.6 & 80.3 & 67.4 & 80.9 & 73.5 & 60.7 & 67.8 & 64.1 & 96.0 & 93.6 & 94.8 & 96.3 & 93.2 & 94.7 \\
         \hline
        \multirow[c]{6}{*}{\rotatebox[origin=c]{90}{LaBSE}} & DInf & 68.4 & 89.7 & 77.6 & 52.6 & 69.5 & 59.9 & 44.3 & 57.3 & 50.0 & 91.1 & 91.1 & 91.1 & 92.5 & 92.5 & 92.5 \\
         & Hun. & 72.4 & 94.9 & 82.1 & 59.3 & 78.2 & 67.5 & 51.9 & 67.0 & 58.5 & 95.7 & 95.7 & 95.7 & 96.8 & 96.8 & 96.8 \\
         & Sink-o & 67.0 & 87.8 & 76.0 & 51.6 & 68.2 & 58.8 & 43.1 & 55.7 & 48.6 & 91.0 & 91.0 & 91.0 & 92.2 & 92.2 & 92.2 \\
         & Sink-d & 72.4 & 94.9 & 82.1 & 59.6 & 78.7 & 67.8 & 52.2 & 67.5 & 58.9 & 95.6 & 95.6 & 95.6 & 97.0 & 97.0 & 97.0 \\
         & SMat & 71.5 & 93.7 & 81.1 & 57.3 & 75.6 & 65.2 & 49.3 & 63.7 & 55.5 & 94.4 & 94.4 & 94.4 & 95.9 & 95.9 & 95.9 \\
         & BMat & 71.5 & 93.7 & 81.1 & 57.3 & 75.6 & 65.2 & 49.3 & 63.7 & 55.5 & 94.4 & 94.4 & 94.4 & 95.9 & 95.9 & 95.9 \\
         \hline
        \multirow[c]{6}{*}{\rotatebox[origin=c]{90}{fastText}} & DInf & 70.3 & 72.9 & 71.6 & 73.7 & 77.0 & 75.3 & 68.4 & 71.8 & 70.1 & 80.9 & 80.9 & 80.9 & 82.7 & 82.7 & 82.7 \\
         & Hun. & 74.9 & 77.6 & 76.2 & 78.1 & 81.5 & 79.8 & 71.2 & 74.7 & 72.9 & 86.1 & 86.1 & 86.1 & 87.8 & 87.8 & 87.8 \\
         & Sink-o & 69.0 & 71.5 & 70.2 & 72.4 & 75.6 & 73.9 & 66.7 & 70.0 & 68.3 & 80.6 & 80.6 & 80.6 & 81.5 & 81.5 & 81.5 \\
         & Sink-d & 74.4 & 77.1 & 75.7 & 77.4 & 80.8 & 79.1 & 71.4 & 74.9 & 73.1 & 84.9 & 84.9 & 84.9 & 87.2 & 87.2 & 87.2 \\
         & SMat & 73.4 & 76.1 & 74.8 & 77.0 & 80.3 & 78.6 & 70.9 & 74.4 & 72.6 & 85.2 & 85.1 & 85.2 & 86.9 & 86.9 & 86.9 \\
         & BMat & 73.4 & 76.1 & 74.8 & 77.0 & 80.3 & 78.6 & 70.9 & 74.4 & 72.6 & 85.2 & 85.1 & 85.2 & 86.9 & 86.9 & 86.9 \\
        \bottomrule
    \end{tabular}
\end{table*}
